# Supplementary material for: Extended-support beta regression for $[0, 1]$ responses
Source: arXiv:2409.07233 source file (2025-05-07)
Supplement: Supplementary file 1 [file xbx-supp-arxiv-0.pdf]

# Supplementary material document for “Extended-support beta regression for $[0, 1]$ responses”

Ioannis Kosmidis 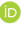\*<sup>1</sup> and Achim Zeileis 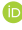†<sup>2</sup>

<sup>1</sup>Department of Statistics, University of Warwick  
Coventry, CV4 7AL, UK

<sup>2</sup>Department of Statistics, University of Innsbruck  
6020 Innsbruck, Austria

September 11, 2024

## S1 Introduction

The supplementary material for “Extended-support beta regression for  $[0, 1]$  responses” is available at <https://github.com/ikosmidis/XBX-supplementary> and provides the current supplementary material document, and instructions and scripts to reproduce all numerical results and figures in the main text and the supplementary material document.

## S2 XBX versus doubly-censored normal distribution

In this section, we carry out a comparison of the XBX distribution to the doubly-censored normal distribution. For each combination of  $\mu \in \{0.5, 0.7, 0.9\}$ ,  $\phi \in \{0.5, 2, 5, 20\}$ , and  $\nu \in \{0.01, 0.1, 1\}$ , we use numerical integration to compute the expected value  $\mu'$  and standard deviation  $\sigma'$  of the  $\text{XBX}(\mu, \phi, \nu)$  distribution. Then, we numerically solve the system of equations

$$\begin{aligned} E(Y' \mid m, s) &= \mu' \\ \sqrt{\text{var}(Y' \mid m, s)} &= \sigma' \end{aligned}$$

with respect  $m$  and  $s$ , where  $Y'$  has a doubly-censored normal distribution in  $(0, 1)$  with mean  $m$  and standard deviation  $s$  for the uncensored Normal distribution. In this way, for each combination of  $\mu$ ,  $\phi$  and  $\nu$ , we can compare XBX and doubly-censored normal distributions that have the same mean and variance. The outcome of the comparison is shown in Figure S1 (densities) and Figure S2 (histograms of samples of size 1000), which can be reproduced using the script `xbx-vs-cn.R` in the supplementary material.

---

\*[ioannis.kosmidis@warwick.ac.uk](mailto:ioannis.kosmidis@warwick.ac.uk)

†[Achim.Zeileis@R-project.org](mailto:Achim.Zeileis@R-project.org)

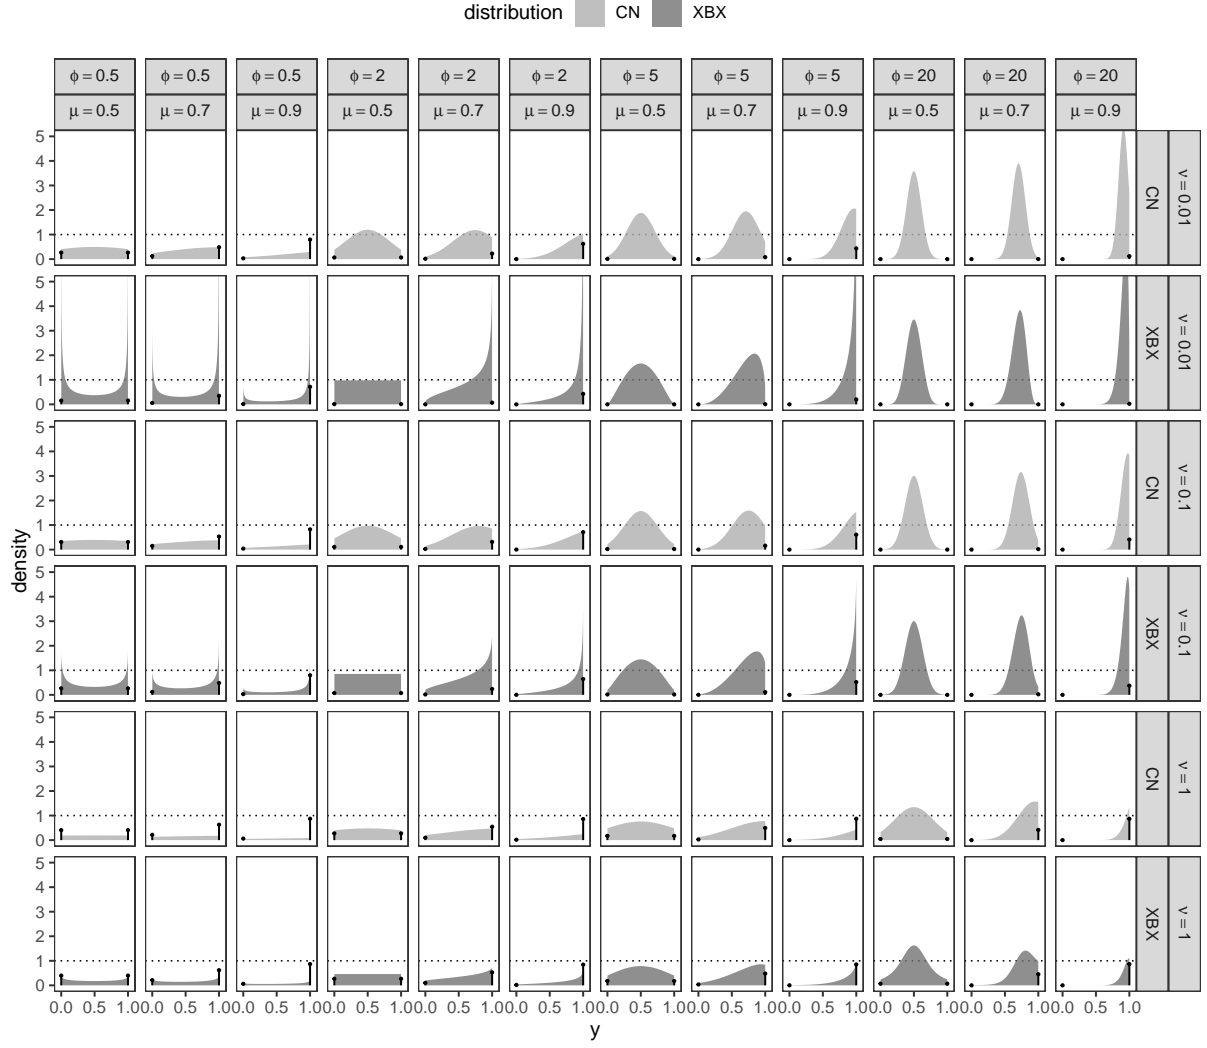

Figure S1: Densities of the XBX distribution (dark grey) and of the doubly-censored normal distribution (light grey) for all combinations of  $\mu \in \{0.5, 0.7, 0.9\}$ ,  $\phi \in \{0.5, 2, 5, 20\}$ , and  $\nu \in \{0.01, 0.1, 1\}$ . The mean and the variance of the doubly-censored normal distribution are numerically matched to be equal to those of the XBX distribution; see Section S2 for details. The horizontal dotted line is at 1.

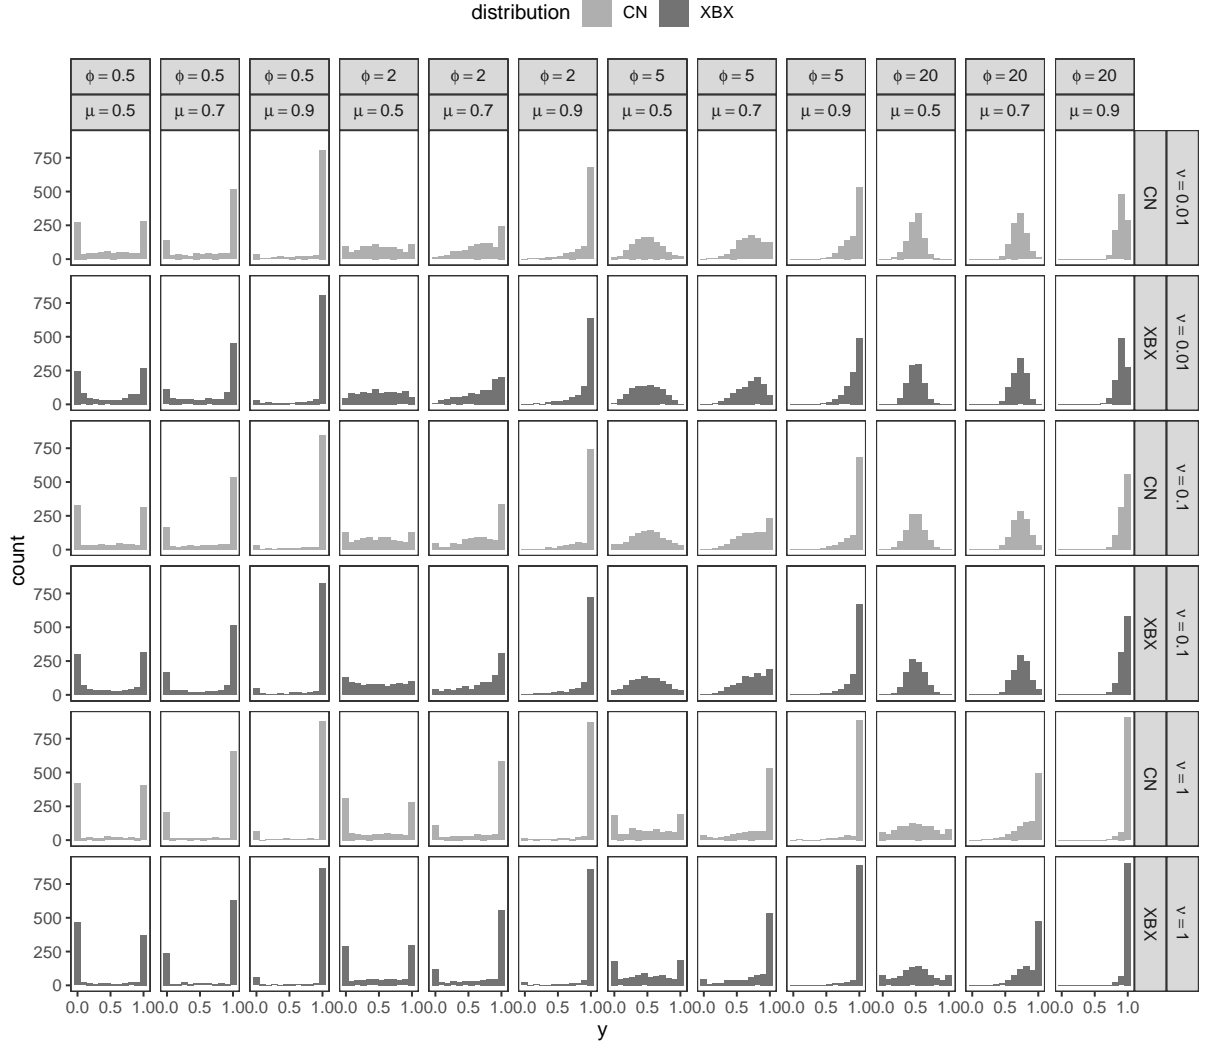

Figure S2: Histograms of samples of size 1000 from the XBX distribution (dark grey) and from the doubly-censored normal distribution (light grey) for all combinations of  $\mu \in \{0.5, 0.7, 0.9\}$ ,  $\phi \in \{0.5, 2, 5, 20\}$ , and  $\nu \in \{0.01, 0.1, 1\}$ . The mean and the variance of the doubly-censored normal distribution are numerically matched to be equal to those of the XBX distribution; see Section S2 for details.

### S3 Supplementary tables and figures for Section 4

In this section, we provide supplementary plots and the full results of the loss aversion analysis in Section 4 of the main text. Specifically, Figure S3 depicts the fitted cumulative distribution functions for every model of Section 4.3, for each level of arrangement, for subjects that are male or teams with at least one male, in grade 10–12 and 16 years of age. The fitted cumulative distributions are contrasted to the corresponding empirical cumulative distribution functions obtained from the subsample of subjects that are male or teams with at least one male, in grades 10–12 and between 15 and 17 years of age. Table S2 and Table S3 show the estimates for the three-part hurdle model of Section 4.7 with a multinomial logistic regression model for the probabilities of boundary and non-boundary observations with the same covariates as those in the linear predictor (16) and predictor (17), respectively, and model B of Section 4.3 for the non-boundary observations.

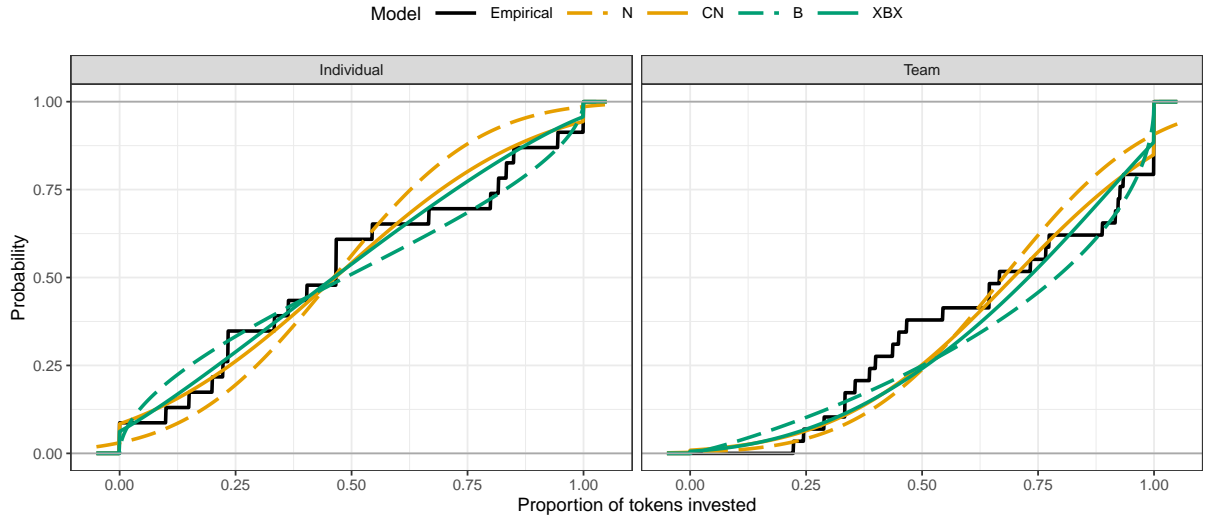

Figure S3: Fitted cumulative distribution functions for every model of Section 4.3 (N, CN, B, XBX), for each level of arrangement, for subjects that are male or teams with at least one male, in grade 10–12 and 16 years of age. The fitted cumulative distributions are contrasted to the corresponding empirical cumulative distribution functions (black) obtained from the subsample of subjects that are male or teams with at least one male, in grades 10–12 and between 15 and 17 years of age.

Table S1: Estimated arrangement effects for subjects that are male or teams with at least one male, in grade 10–12 and 16 years of age. The rows for  $P(Y < 0.05)$  show model-based estimates of the probability to invest less than 5% of the tokens. All effects are contrasted to the corresponding empirical quantities obtained from the subsample of subjects that are male or teams with at least one male, in grades 10–12, and between 15 and 17 years of age. The rows for the parameters show the estimates of the distributional parameters for each arrangement setting.

|               | Arrangement | Empirical | N        | CN    |       | B      | XBX   |       |
|---------------|-------------|-----------|----------|-------|-------|--------|-------|-------|
| $P(Y < 0.05)$ | Individual  | 0.087     | 0.047    | 0.109 |       | 0.135  | 0.102 |       |
|               | Team        | 0         | 0.006    | 0.014 |       | 0.015  | 0.011 |       |
| Parameters    | Individual  |           | $\mu$    | 0.461 | 0.465 | $\mu$  | 0.492 | 0.475 |
|               |             |           | $\sigma$ | 0.246 | 0.337 | $\phi$ | 1.091 | 2.602 |
|               |             |           |          |       |       | $\nu$  |       | 0.103 |
|               | Team        |           | $\mu$    | 0.675 | 0.696 | $\mu$  | 0.700 | 0.662 |
|               |             |           | $\sigma$ | 0.246 | 0.294 | $\phi$ | 1.637 | 3.602 |
|               |             |           |          |       |       | $\nu$  |       | 0.103 |

Table S2: Coefficient estimates, estimated standard errors (in parentheses), maximized log-likelihood, AIC, and BIC for the three-part hurdle, with a multinomial logistic regression model for the probabilities of boundary and non-boundary observations with the same covariates as those in the linear predictor (16), and the beta regression model B for the non-boundary observations; see Section 4.7. Estimates for the multinomial regression part have been obtained using the VGAM R package Yee (2010); the standard errors that are greater than 1000 are in reality infinite due to separation, as are the corresponding estimates.

|                                        | Zero-and-one-inflated beta |                         |                     |                   |
|----------------------------------------|----------------------------|-------------------------|---------------------|-------------------|
|                                        | $\log(\pi_0/\pi_{0,1})$    | $\log(\pi_1/\pi_{0,1})$ | $\text{logit}(\mu)$ | $\log(\phi)$      |
| (Intercept)                            | -22.192<br>(14 749.887)    | -23.232<br>(10.334)     | -0.858<br>(0.597)   | 1.209<br>(0.087)  |
| $G_i$ (Grade)                          | 22.265<br>(14 749.888)     | 11.526<br>(10.841)      | -2.195<br>(1.102)   | 0.222<br>(0.115)  |
| $T_i$ (Arrangement)                    | -0.379<br>(2642.760)       | -0.744<br>(0.960)       | 0.278<br>(0.112)    | 0.422<br>(0.131)  |
| $A_i$ (Age)                            | 0.060<br>(1158.335)        | 1.361<br>(0.753)        | 0.045<br>(0.047)    |                   |
| $S_i$ (Sex)                            | 0.759<br>(0.759)           | 1.885<br>(0.549)        | 0.318<br>(0.089)    | -0.292<br>(0.122) |
| $G_i T_i$ (Grade $\times$ Arrangement) | -1.057<br>(2642.760)       | 1.539<br>(1.053)        | 0.448<br>(0.171)    |                   |
| $G_i A_i$ (Grade $\times$ Age)         | -0.264<br>(1158.335)       | -0.885<br>(0.777)       | 0.112<br>(0.072)    |                   |
| Log-likelihood                         |                            |                         |                     | -46.5             |
| AIC                                    |                            |                         |                     | 143.0             |
| BIC                                    |                            |                         |                     | 251.6             |

Table S3: Coefficient estimates, estimated standard errors (in parentheses), maximized log-likelihood, AIC, and BIC for the three-part hurdle, with a multinomial logistic regression model for the probabilities of boundary and non-boundary observations with the same covariates as those in the linear predictor (17), and the beta regression model B for the non-boundary observations; see Section 4.7. Estimates for the multinomial regression part have been obtained using the VGAM R package Yee (2010); the standard errors that are greater than 1000 are in reality infinite due to separation, as are the corresponding estimates.

|                                        | Zero-and-one-inflated beta |                         |                     |                   |
|----------------------------------------|----------------------------|-------------------------|---------------------|-------------------|
|                                        | $\log(\pi_0/\pi_{0,1})$    | $\log(\pi_1/\pi_{0,1})$ | $\text{logit}(\mu)$ | $\log(\phi)$      |
| (Intercept)                            | -21.156<br>(1225.251)      | -5.671<br>(0.634)       | -0.858<br>(0.597)   | 1.209<br>(0.087)  |
| $G_i$ (Grade)                          | 17.840<br>(1225.251)       | 2.263<br>(0.506)        | -2.195<br>(1.102)   | 0.222<br>(0.115)  |
| $T_i$ (Arrangement)                    | -1.430<br>(1.130)          | 0.425<br>(0.428)        | 0.278<br>(0.112)    | 0.422<br>(0.131)  |
| $A_i$ (Age)                            |                            |                         | 0.045<br>(0.047)    |                   |
| $S_i$ (Sex)                            | 0.919<br>(0.758)           | 1.880<br>(0.541)        | 0.318<br>(0.089)    | -0.292<br>(0.122) |
| $G_i T_i$ (Grade $\times$ Arrangement) |                            |                         | 0.448<br>(0.171)    |                   |
| $G_i A_i$ (Grade $\times$ Age)         |                            |                         | 0.112<br>(0.072)    |                   |
| Log-likelihood                         |                            |                         |                     | -53.5             |
| AIC                                    |                            |                         |                     | 145.1             |
| BIC                                    |                            |                         |                     | 227.7             |

## S4 XBX versus heteroscedastic two-limit tobit regression

In this section, we provide supplementary plots and the full results of the simulation experiment in Section 5 of the main text, for the comparison of XBX regression with heteroscedastic two-limit tobit regression model in terms of their predictive performance. Specifically, Figure S4 to Figure S7 show simulated data sets for all combinations of  $u \in \{2^{-6}, 2^{-5}, \dots, 2\}$ , and  $[\mu_1, \mu_n]$  and  $[\phi_1, \phi_n]$  in Table 4. Figure S8 shows the average relative change in  $S$ ,  $S_{\text{HT}}/S_{\text{XBX}} - 1$ , as a function of  $u$ , when moving from XBX regression to the two-limit heteroscedastic tobit, based on their maximum likelihood fits, for all combinations of  $[\mu_1, \mu_n]$  and  $[\phi_1, \phi_n]$  in Table 4.

The simulation experiment, Figure S4 to Figure S7, Figure S8, and Figure 6 in the main text can be reproduced using the script `xbx-vs-htobit-crss.R` in the supplementary material.

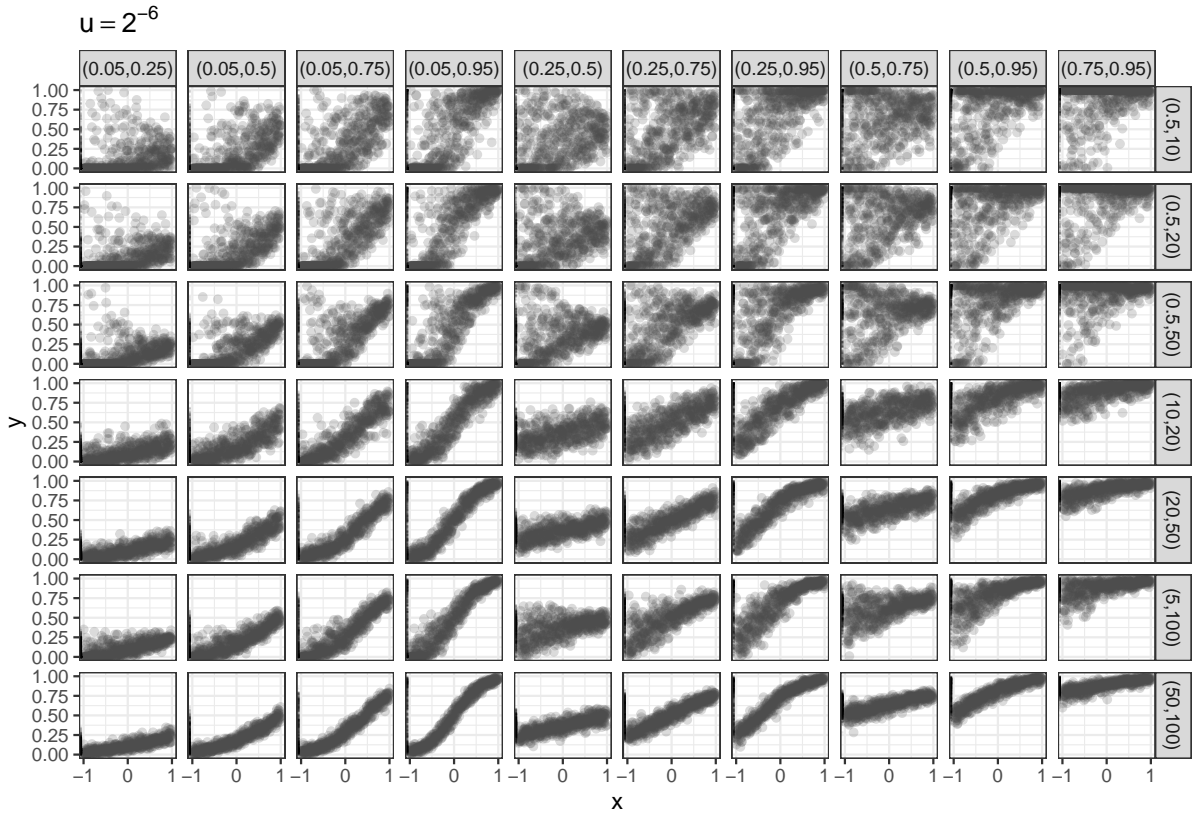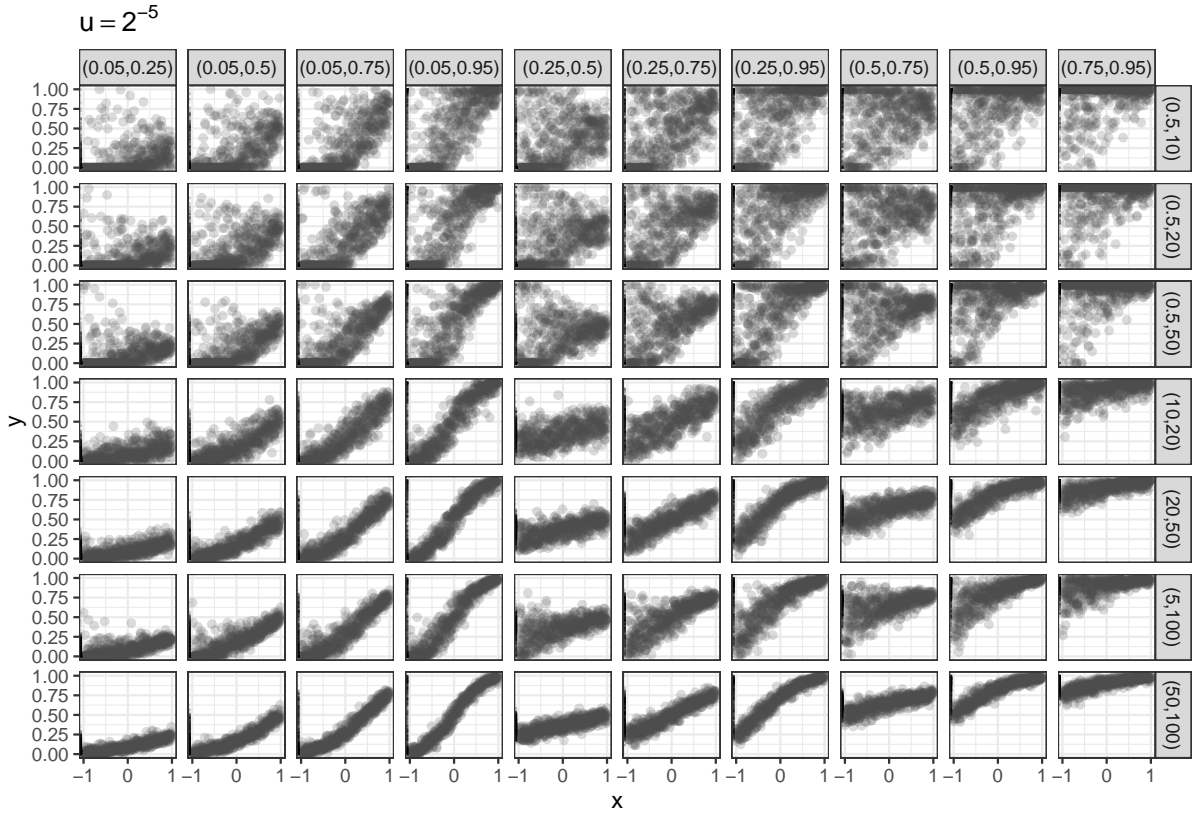

Figure S4: Scatterplots of simulated response ( $y$ ) versus covariate ( $x$ ) values for  $u = 2^{-6}$  and  $u = 2^{-5}$ , for all combinations of  $[\mu_1, \mu_n]$  and  $[\phi_1, \phi_n]$  in Table 4 of the main text.

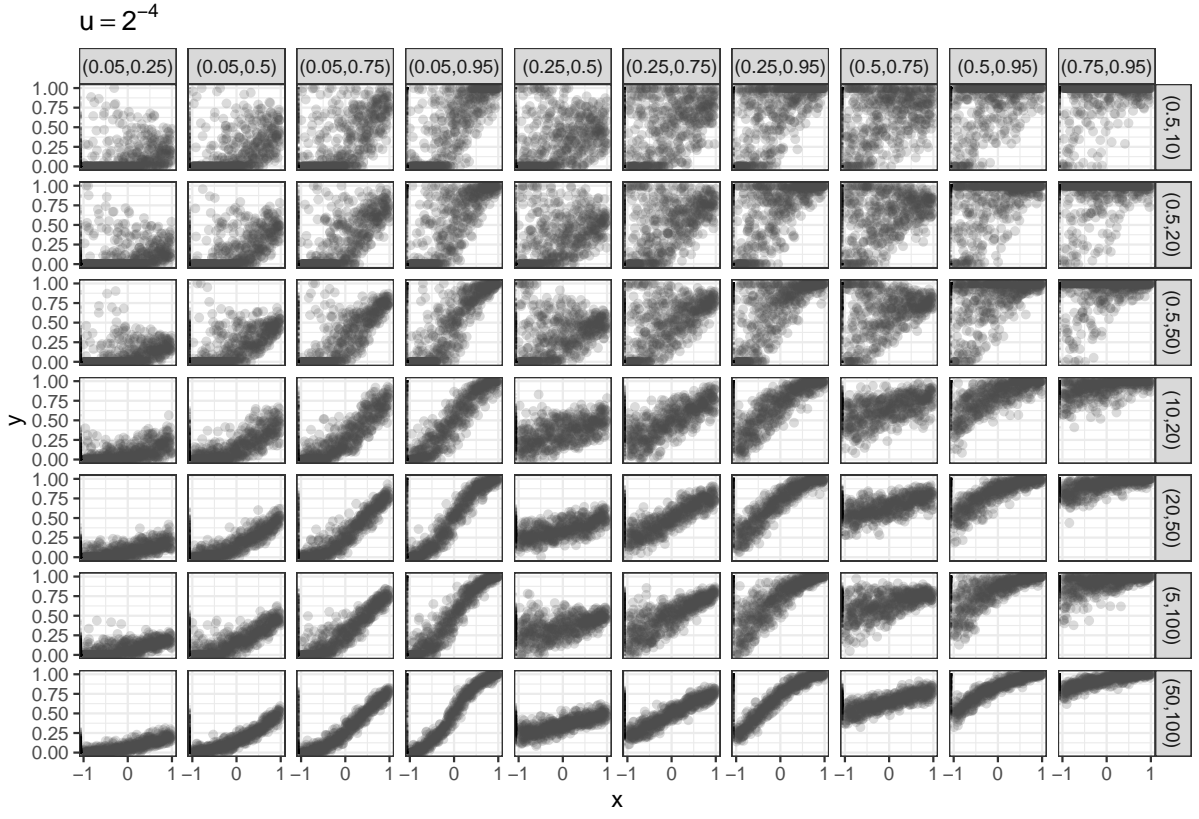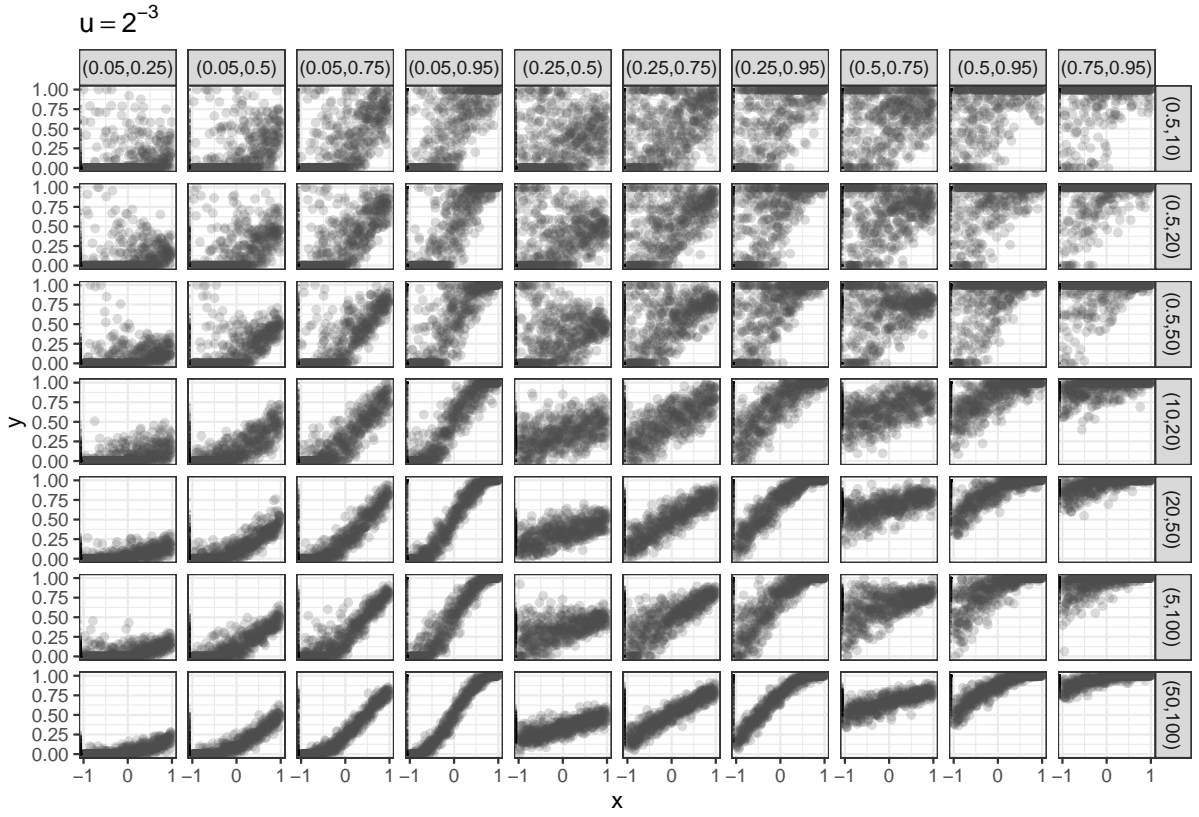

Figure S5: Scatterplots of simulated response ( $y$ ) versus covariate ( $x$ ) values for  $u = 2^{-4}$  and  $u = 2^{-3}$ , for all combinations of  $[\mu_1, \mu_n]$  and  $[\phi_1, \phi_n]$  in Table 4 of the main text.

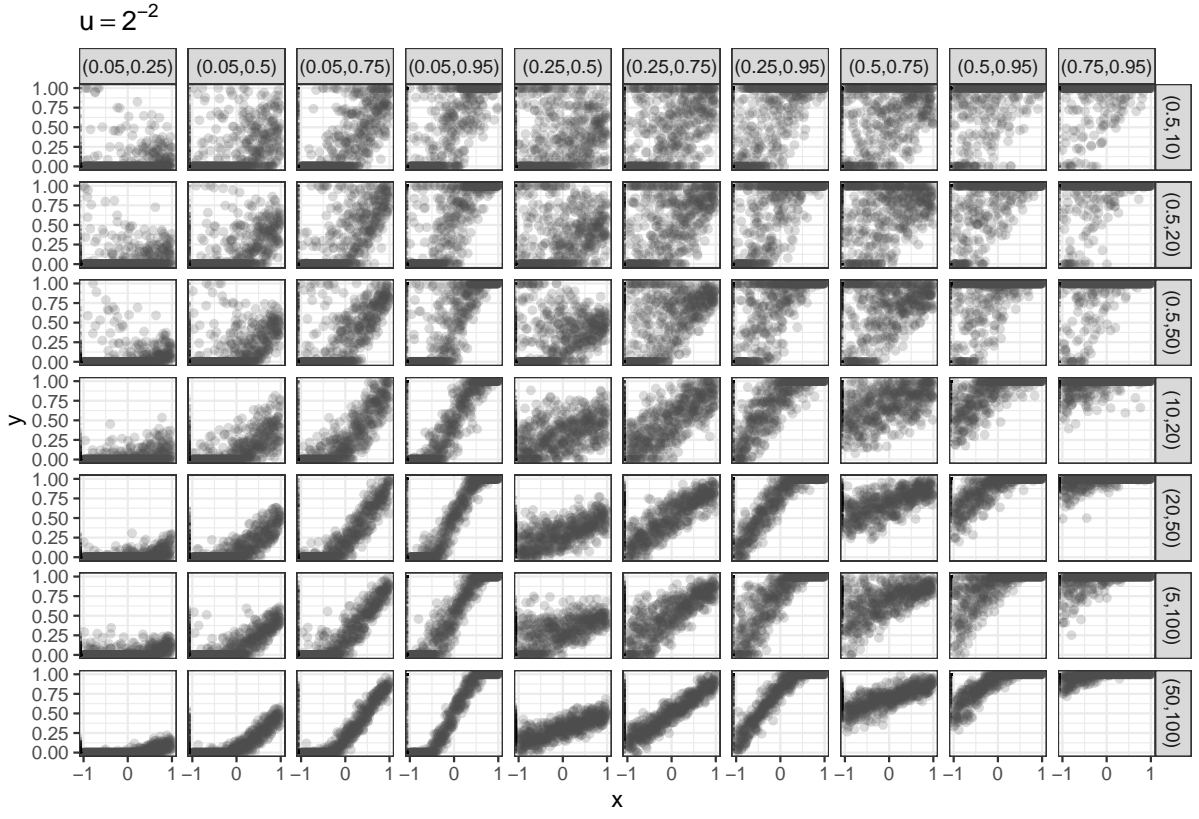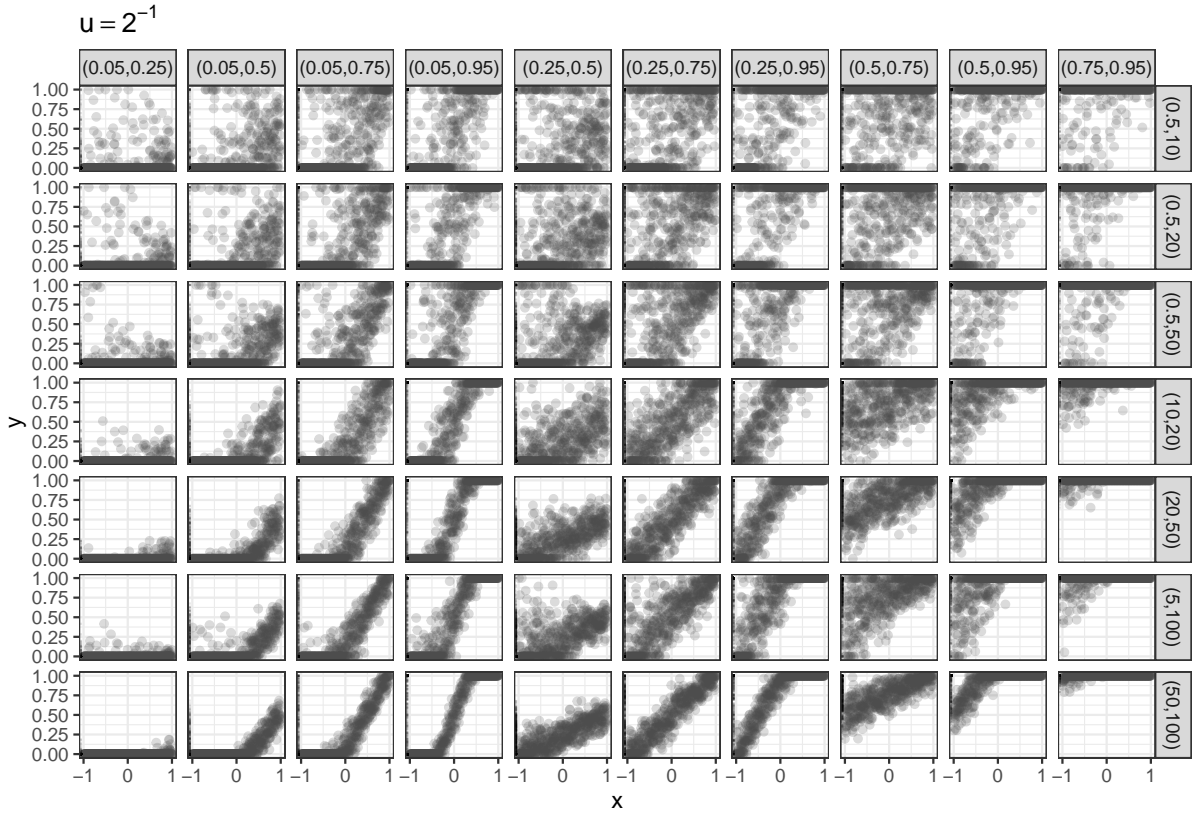

Figure S6: Scatterplots of simulated response ( $y$ ) versus covariate ( $x$ ) values for  $u = 2^{-2}$  and  $u = 2^{-1}$ , for all combinations of  $[\mu_1, \mu_n]$  and  $[\phi_1, \phi_n]$  in Table 4 of the main text.

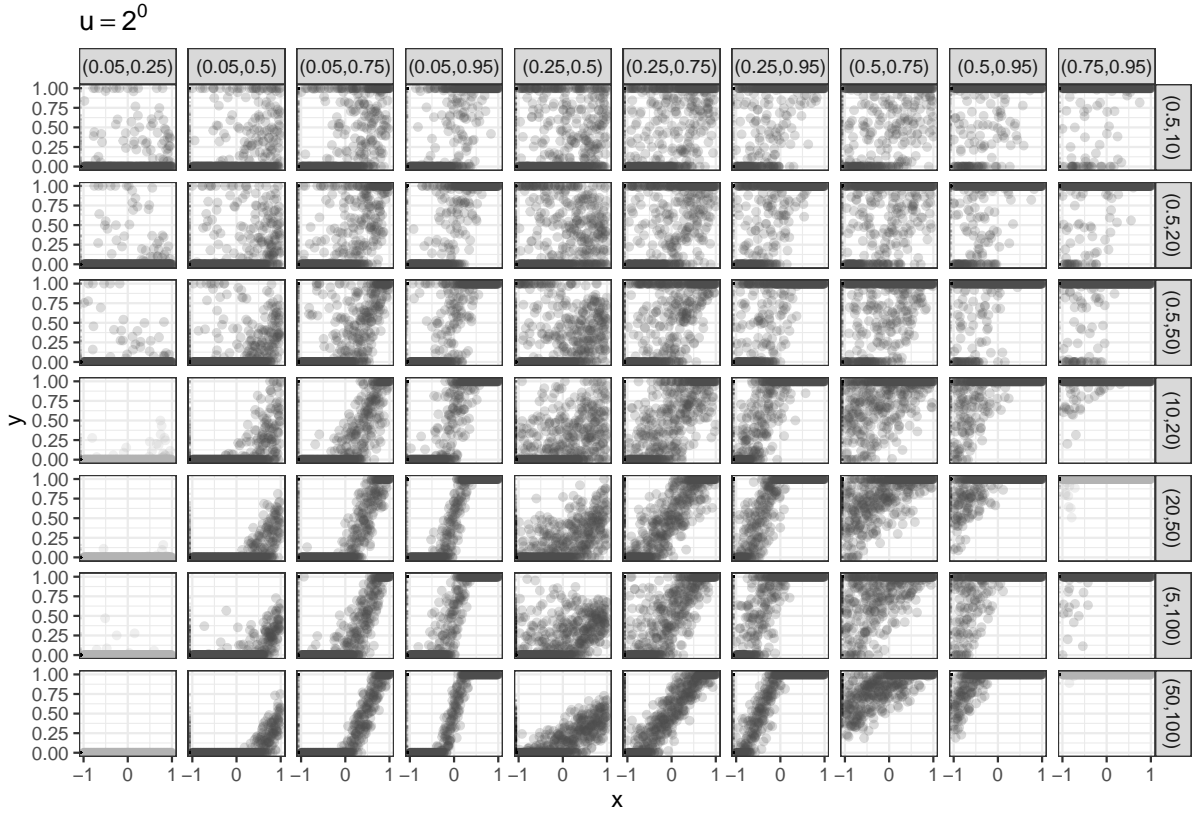

Figure S7: Scatterplots of simulated response ( $y$ ) versus covariate ( $x$ ) values for  $u = 1$  and  $u = 2$ , for all combinations of  $[\mu_1, \mu_n]$  and  $[\phi_1, \phi_n]$  in Table 4 of the main text. Light grey indicates settings where the average probability of boundary observations is larger than 0.95.

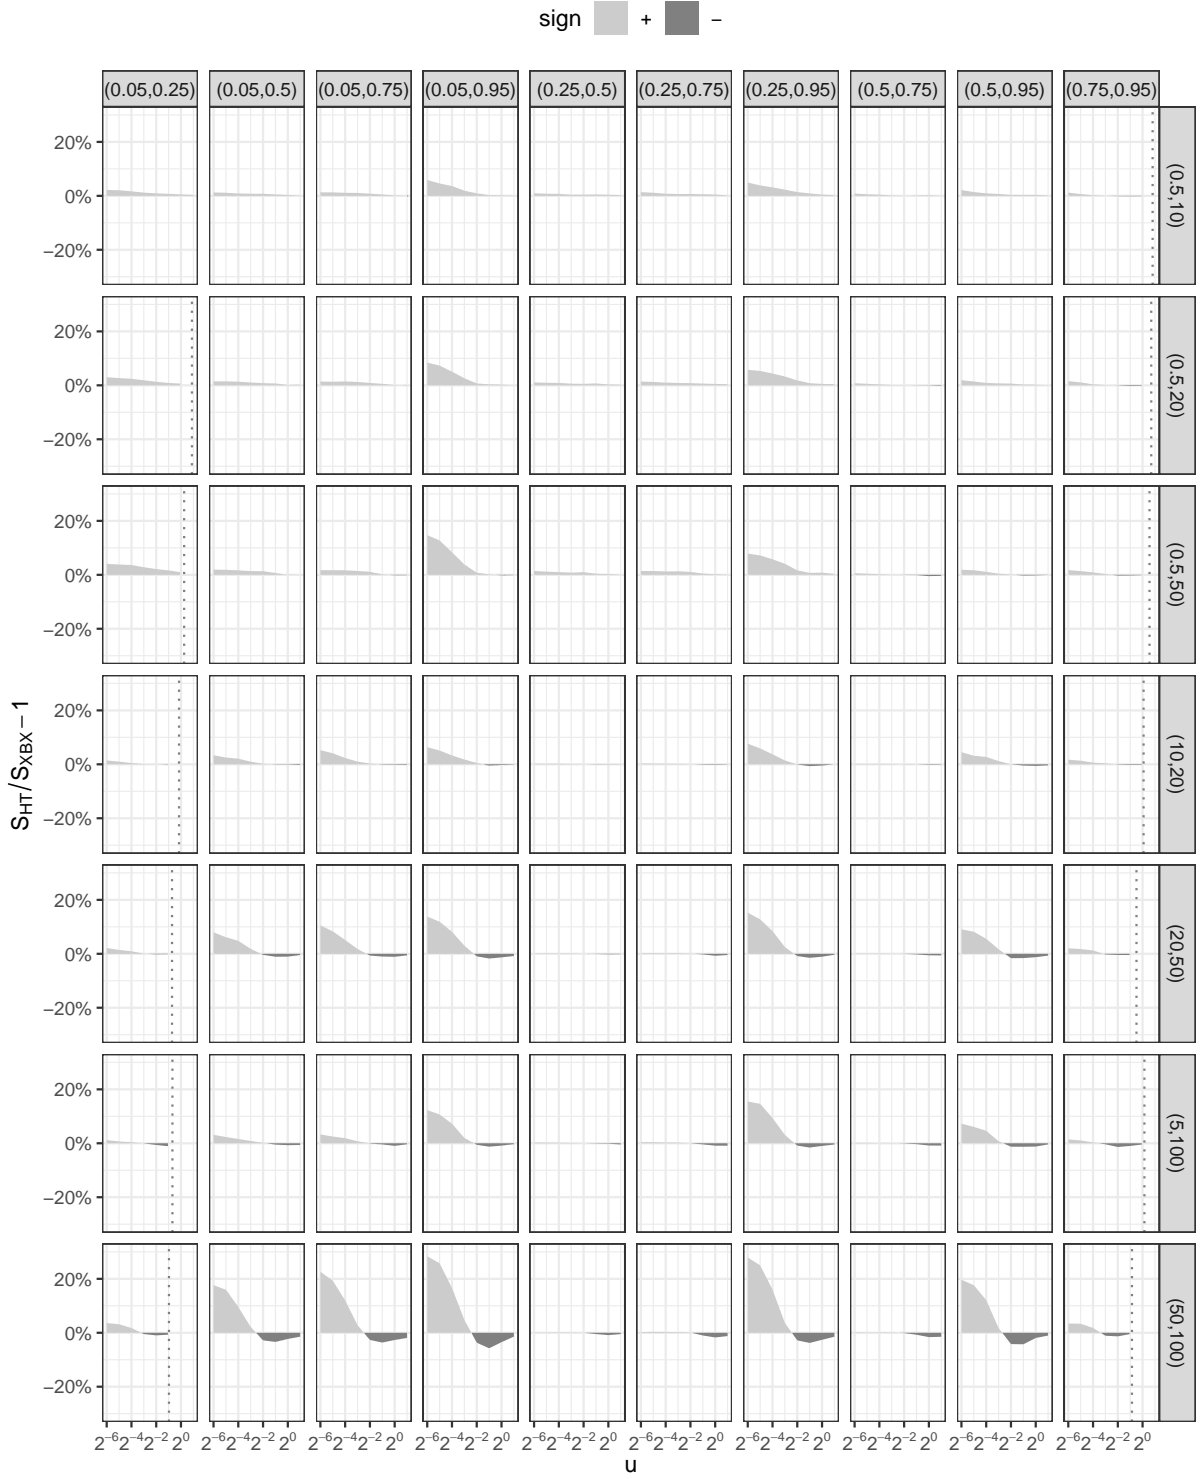

Figure S8: Average relative change in  $S$  when moving from XBX regression to the two-limit heteroscedastic model, based on 100 samples of size  $n = 500$  for each combination of  $u \in \{2^{-6}, 2^{-5}, \dots, 2\}$ , and  $[\mu_1, \mu_n]$  (columns) and  $[\phi_1, \phi_n]$  (rows) intervals in Table 4. The dotted vertical lines are the smallest values of  $u$  for which the average probability of boundary observations exceeds 0.95 for each combination of  $[\mu_1, \mu_n]$  and  $[\phi_1, \phi_n]$ .

## References

Yee TW (2010). “The VGAM Package for Categorical Data Analysis.” *Journal of Statistical Software*, **32**(10), 1–34. doi:10.18637/jss.v032.i10.
